# Supplementary material for: Revisiting Safe Exploration in Safe Reinforcement learning
Source: arXiv:2409.01245 source file (2024-09-02)
Supplement: Supplementary file 1 [file 8_Appendix.tex]

The Circle2D environment is designed to be flexible in its configuration and simple to extent and customize.
We expose the configuration parameters in Tab.\ref{tab:EnvironmentConfigParameter} for customization of the environment.
